# Supplementary material for: Premonition Net, A Multi-Timeline Transformer Network Architecture Towards Strawberry Tabletop Yield Forecasting
Source: arXiv:2211.08177 source file (2022-11-15)
Supplement: Supplementary file 1 [file appendix.tex]

\appendices
\section{}
% \section{Proof of the First Zonklar Equation}
% Appendix one text goes here.

% you can choose not to have a title for an appendix
% if you want by leaving the argument blank
% \section{}
% Appendix two text goes here.
